# Supplementary material for: Scalable, Validated Code Translation of Entire Projects using Large Language Models
Source: arXiv:2412.08035 source file (2024-12-11)
Supplement: Supplementary file 1 [file appendix.tex]

\appendix
\section*{Appendix}

\section{Mapping Go interfaces to Rust traits}

The corresponding feature mapping rule is (Map-Interface) in \autoref{fig:interface-mapping}. 

For a source Go project $P$, we collect the set of all method signatures that appear in interfaces using $\textbf{interfaceMethods}(P)$. We incrementally build a mapping \textbf{gadgettrait} from a method signature in $\textbf{interfaceMethods}(P)$ to a unique Rust gadget-trait.
During translation of an interface, we check whether a method signature already has a corresponding gadget-trait and reuse if so. Moreover, we maintain a mapping \textbf{supertraits} from a Go interface to Rust traits translated from its super-interface (e.g. the super traits for \gocode{Batcher} is \rustcode{canValidate}).

% {\textbf{\hlz{This paragraph is for discussion and may need to be deleted.}}} The features mapping rule for interface requires a well-defined translation order so that we always translate super interfaces first (e.g. \gocode{canValidate} in this example). This is possible if the orignal Go code does not contain two interfaces that have exactly the same method set, and that interfaces do not reference each other. A short reasoning for this: if interfaces are unique, then the set of all interfaces $\{I\}$ can be treated as a subset of $2^{\textbf{interfaceMethods}(P)}$ (the set of all subsets of all interface methods). $2^{\textbf{interfaceMethods}(P)}$ forms a lattice under set-containment relation, which is directed acyclic graph. Now since $\{I\}$ is a subset of it, it should be a directed acyclic graph too. In this case, we can define the translation order to be the postorder of this DAG.

% Note that the above target feature does not fully account for the structurality of \textcolor{Go}{Go} \gocode{interface}. In case the source program $P$ contains overlapping interfaces (i.e. interfaces that share same methods), we need to further avoid duplication of sub-traits. To achieve this, we compute all method signatures appeared in interfaces $\textbf{interfaceMethods}(P)$ as defined in ~\autoref{fig:golang-aux}. During translation of an \gocode{interface}, we check whether a method signature already has a corresponding sub trait generated by maintaining a mapping $\textbf{subtrait}$ from method signature to sub-trait.

\begin{figure}[h]
\centering
\small 
\[
\begin{array}{cc}
\irule{
\begin{array}{c}
    \gocode{Id}: \gocode{type}\ I\ \gocode{interface}\ \{ \overline{f\ S} \} \in P \\
    \overline{h\ T} = \left\{h\ T\middle| h\ T \in \overline{f\ S} \land h\ T \in \textbf{gadgettrait}\right\} \land \overline{K_h} = \textbf{gadgettrait}(\overline{h\ T}) \\ 
    \overline{L} = \textbf{supertraits}(\gocode{Id})\\
    \gocode{Id}: \gocode{type}\ I\ \gocode{interface}\ \{ \overline{f\ S} \setminus \overline{h\ T} \} \rightsquigarrow_{\text{LLM}} \rustcode{code}
\end{array}
}{
\rustcode{code} \Downarrow \rustcode{trait}\ J\ \{\overline{\rustcode{fn}\ g\ S_m}\} \vdash \gocode{Id} \mapsto
\begin{array}{c}
    \rustcode{trait}\ J: \overline{J_g} + \overline{K_h} + \overline{L}\ \{\}\ \ \overline{\rustcode{trait}\ J_g\ \{\rustcode{fn}\ g\ S_m\}} \\
    \rustcode{impl<}T\rustcode{>}\ J\ \rustcode{for}\ T\ \rustcode{where}\ T: \overline{J_g} + \overline{K_h} \{\}
\end{array}
} & (\text{Map-Interface})\\ \\ 
\irule{
\begin{array}{c}
    f\ S \in \textbf{interfaceMethods}(P) \land I = \textbf{gadgettrait}(f\ S) \land \textbf{rustSignature}(I) = \rustcode{fn}\ g\ S_m \\
    \gocode{Id}: \gocode{func}\ (t\ T)\ f\ S\ \{\dots\}
    \rightsquigarrow_{\text{LLM}} \rustcode{code}
\end{array}
}{
\begin{array}{c}
    \rustcode{code} \Downarrow \rustcode{impl}\ U\ \{\ \rustcode{fn}\ g\ S_m\ \{\dots\} \ \} \\ 
    \vdash \gocode{Id} \mapsto \rustcode{impl}\ I\ \rustcode{for}\ U\ \{\ \rustcode{fn}\ g\ S_m\ \{\dots\} \ \}
\end{array}
% \texttt{\color{Rust} e} \Downarrow \texttt{\color{Rust} impl T' \{ fn f'(self, x') \{...\}\}} \vdash \texttt{\color{Go}Id} \mapsto \texttt{\color{Rust} impl Im for T' \{ fn f'(self, x') \{...\}\}}
} & (\text{Map-Impl-Interface})\\ \\ 
\end{array}
\]
\caption{Mapping interfaces to traits}
\label{fig:interface-mapping}
\end{figure}
 Rule (Map-Interface) requires of post-processing (corresponding to \textbf{PostProcessing} in Algorithm~\ref{alg:feature-mapping}). Instead of requesting the complex target feature described above, we construct a prompt that queries for a trivial translation (i.e. a \rustcode{trait}) for the original \gocode{interface}. Then, we process the LLM's response  and decompose the generated \rustcode{trait} into multiple sub-traits. If some methods (e.g. $\overline{h\ T}$) of this \gocode{interface} already have corresponding sub-traits defined (e.g. $\overline{K_h}$), we exclude them from the query and reuse the existing sub-traits. Note that we synthesise the names denoted by $J_g$. For example, the sub-trait name \rustcode{Batcher\_Validate} is generated by us from the trait name \rustcode{Batcher} and the method name \rustcode{Validate}.

Rule (Map-Impl-Interface) in Figure~\ref{fig:interface-mapping} captures the generation of translations for methods that implement interfaces. In such cases, we specifically instruct the LLMs to generate methods whose signature is consistent with the method signature in the corresponding sub-trait. Again, instead of requesting a more complex impl-trait, we construct a prompt to query for a normal method, and instrument the generated code as part of \textbf{PostProcessing}.

% \subsubsection{Lazy subtrait generation}\hlz{Only if we have rooms}
% \subsubsection{Method Delegation}
% \begin{figure}[h]
% \centering
% \small 
% \[
% \begin{array}{cc}
% \irule{
% \begin{array}{c}
%     f\ S \in \textbf{interfaceMethods}(P) \land I = \textbf{subtrait}(f\ S) \land \textbf{rustSignature}(I) = \rustcode{fn}\ g\ S_m \\
%     \gocode{Id1}: \gocode{type}\ T\ \gocode{struct} \{\ U, \dots\ \} \in P \land
%     \gocode{Id2}: \gocode{func}\ (t\ U)\ f\ S\ \{\dots\} \in P
%     % \rightsquigarrow_{\text{LLM}} \rustcode{code}
% \end{array}
% }{
% \begin{array}{c}
%     \vdash \gocode{Id} \mapsto \rustcode{impl}\ I\ \rustcode{for}\ T\ \{\ \rustcode{fn}\ g\ S_m\ \{\dots\} \ \}
% \end{array}
% } & (\text{Method-Delegation})\\ \\ 
% \end{array}
% \]
% \caption{Method Delegation}
% \label{fig:method-delegation}
% \end{figure}
